# Supplementary material for: Bridging Spectral-wise and Multi-spectral Depth Estimation via Geometry-guided Contrastive Learning
Source: arXiv:2503.00793 source file (2025-03-02)
Supplement: Supplementary file 1 [file 07_supple.tex]

\section{Appendix}
In this supplementary material, we provide

\begin{itemize}
\item 
Further analysis of ablation study.
\item 
Discussion and future plan.
\end{itemize}

\section{Ablation Study}
We further provide the ablation study of the main paper, as shown in~\cref{tab:ablation3} and~\cref{tab:ablation4}.
The two tables show that, in general, feature fusion brings a significant performance improvement for each modality in challenging environments.   
It compensates for the weaknesses of each sensor, low-light sensitivity in night conditions (\ie, RGB camera), occlusion and blur effects in rainy conditions (\ie, RGB and NIR cameras), and insufficient texture and contrast in general conditions (\ie, thermal camera).
However, in environments where each sensor is fully functional, such as daytime conditions with clear-sky for RGB and NIR sensors, sensor fusion may not yield performance improvement.

\begin{table}[t]
\centering
\caption{\textbf{The effect of multi-spectral feature fusion for various environments (NIR).}  
To investigate the effect of multi-spectral feature fusion under each environmental condition, we compare evaluation results (\ie, Day, Night, and Rain).
GT depth maps projected to the NIR image plane are used for evaluation.
} \vspace{-0.1in}
\begin{center}
\resizebox{0.99\linewidth}{!}
{
    
    \footnotesize
    \begin{tabular}{c|c|c|c|cc} 
    \toprule
    \multirow{2}{*}{Method} & \multirow{2}{*}{Modal} & \multirow{2}{*}{TestSet} & \multirow{2}{*}{RMSE ($\downarrow)$} & \multicolumn{2}{c}{\textbf{Accuracy $\uparrow$}} \\ \cline{5-6}
     & & & & $\delta < 1.25$ & $\delta<1.25^2$ \\
    \hline 
    %  \multirow{4}{*}{NewCRF +\textit{align}} & \multirow{4}{*}{\rotatebox{90}{RGB}} 
        &  \multirow{4}{*}{\rotatebox{90}{NIR}} 
                          & Day   & 2.938 & 0.941 & 0.994 \\ 
        NeWCRF          & & Night & 2.937 & 0.922 & 0.994 \\ 
        +\textit{align} & & Rain  & 4.873 & 0.829 & 0.963 \\  \cline{3-6}
        & & \cellcolor{Gray1}Avg  & \cellcolor{Gray1}3.617 & \cellcolor{Gray1}0.896 & \cellcolor{Gray1}0.983 \\
    \midrule  
    %  \multirow{4}{*}{NewCRF +\textit{fuse}} & \multirow{4}{*}{\rotatebox{90}{RGB}} 
        & \multirow{4}{*}{\rotatebox{90}{NIR}} 
                         & Day   & 2.889 (\textcolor{red}{-0.049}) & 0.944 (\textcolor{red}{+0.003}) & 0.995 (\textcolor{red}{+0.001}) \\
        NeWCRF         & & Night & 2.840 (\textcolor{red}{{-0.097}}) & 0.931 (\textcolor{red}{{+0.009}}) & 0.994 (\textcolor{red}{{+0.000}}) \\
        +\textit{fuse}  & & Rain  & 3.975 (\textcolor{red}{\textbf{-0.898}}) & 0.879 (\textcolor{red}{\textbf{+0.050}}) & 0.981 (\textcolor{red}{\textbf{+0.018}}) \\ \cline{3-6}
        & & \cellcolor{Gray1}Avg  & \cellcolor{Gray1}3.255 (\textcolor{red}{-0.362})  & \cellcolor{Gray1}0.917 (\textcolor{red}{+0.021}) & \cellcolor{Gray1}0.990 (\textcolor{red}{+0.007}) \\
    \bottomrule
    \end{tabular} 
}
\end{center}
\label{tab:ablation3}
\end{table}

\begin{table}[t]
\centering
\caption{\textbf{The effect of multi-spectral feature fusion for various environments (Thermal).}  
To investigate the effect of multi-spectral feature fusion under each environmental condition, we compare evaluation results (\ie, Day, Night, and Rain).
GT depth maps projected to the thermal image plane are used for evaluation.
} \vspace{-0.1in}
\begin{center}
\resizebox{0.99\linewidth}{!}
{
    
    \footnotesize
    \begin{tabular}{c|c|c|c|cc} 
    \toprule
    \multirow{2}{*}{Method} & \multirow{2}{*}{Modal} & \multirow{2}{*}{TestSet} & \multirow{2}{*}{RMSE ($\downarrow)$} & \multicolumn{2}{c}{\textbf{Accuracy $\uparrow$}} \\ \cline{5-6}
     & & & & $\delta < 1.25$ & $\delta<1.25^2$ \\
    \hline 
    %  \multirow{4}{*}{NewCRF +\textit{align}} & \multirow{4}{*}{\rotatebox{90}{RGB}} 
        &  \multirow{4}{*}{\rotatebox{90}{THR}} 
                          & Day   & 2.671 & 0.954 & 0.995 \\ 
        NeWCRF          & & Night & 2.519 & 0.951 & 0.996 \\ 
        +\textit{align} & & Rain  & 3.349 & 0.916 & 0.990 \\  \cline{3-6}
        & & \cellcolor{Gray1}Avg  & \cellcolor{Gray1}2.860 & \cellcolor{Gray1}0.940 & \cellcolor{Gray1}0.994 \\
    \midrule  
    %  \multirow{4}{*}{NewCRF +\textit{fuse}} & \multirow{4}{*}{\rotatebox{90}{RGB}} 
        & \multirow{4}{*}{\rotatebox{90}{THR}} 
                         & Day   & 2.452 (\textcolor{red}{\textbf{-0.219}}) & 0.964 (\textcolor{red}{\textbf{+0.010}}) & 0.997 (\textcolor{red}{+0.002}) \\
        NeWCRF         & & Night & 2.424 (\textcolor{red}{{-0.095}}) & 0.960 (\textcolor{red}{{+0.009}}) & 0.998 (\textcolor{red}{{+0.002}}) \\
        +\textit{fuse}  & & Rain  & 2.964 (\textcolor{red}{\textbf{-0.385}}) & 0.939 (\textcolor{red}{\textbf{+0.023}}) & 0.994 (\textcolor{red}{\textbf{+0.004}}) \\ \cline{3-6}
        & & \cellcolor{Gray1}Avg  & \cellcolor{Gray1}2.623 (\textcolor{red}{-0.237})  & \cellcolor{Gray1}0.954 (\textcolor{red}{+0.014}) & \cellcolor{Gray1}0.996 (\textcolor{red}{+0.002}) \\
    \bottomrule
    \end{tabular} 
}
\end{center}
\label{tab:ablation4}
\end{table}

\section{Discussion\&Future Plan}
\textbf{Additional Sensor Modality.}
In this paper, we currently aim to learn shared representation between multi-spectrum modalities (\eg, RGB, NIR, and thermal spectrum bands) for the monocular depth estimation task.
However, we could consider additional modalities such as LiDAR and Radar to resolve the scale-ambiguity problem and to get metric-scale depth accuracy.
Also, the data of LiDAR and Radar can be represented as sparse 3d point clouds or image-like projected depth maps.
It is also an interesting topic about which representation is a more suitable form to integrate with our proposed method.
Therefore, we plan to extend our proposed method to include LiDAR or Radar modality for robust and accurate depth estimation.

\textbf{Effective Attention Mask Generation.}
Currently, as described in Sec.3.3 of the main paper, we utilize one prior knowledge that the thermal spectrum domain generally has strong reliability and robustness against various adverse weather conditions.
Therefore, we calculate the attention mask based on the spectrum-shared feature of the thermal image.
However, we cannot use this method when the thermal image is not available or unreliable in some cases, such as temporal disconnection by Non-Uniformity Correction (NUC) operation, lens occlusion, or hardware problems.
Therefore, we need another attention mask generation method, such as relying on depth map consistency of each spectrum image or cross feature-map consistency between each spectrum-shared feature.
We plan to study more effective attention mask generation methods and fusion strategies.
