# Supplementary material for: Bridging Spectral-wise and Multi-spectral Depth Estimation via Geometry-guided Contrastive Learning
Source: arXiv:2503.00793 source file (2025-03-02)
Supplement: Supplementary file 2 [file 04_supple_abl.tex]

\begin{table}[t]
\centering
\caption{\textbf{The effect of multi-spectral feature fusion for various environments (NIR).}  
To investigate the effect of multi-spectral feature fusion under each environmental condition, we compare evaluation results (\ie, Day, Night, and Rain).
GT depth maps projected to the NIR image plane are used for evaluation.
} \vspace{-0.1in}
\begin{center}
\resizebox{0.99\linewidth}{!}
{
    
    \footnotesize
    \begin{tabular}{c|c|c|c|cc} 
    \toprule
    \multirow{2}{*}{Method} & \multirow{2}{*}{Modal} & \multirow{2}{*}{TestSet} & \multirow{2}{*}{RMSE ($\downarrow)$} & \multicolumn{2}{c}{\textbf{Accuracy $\uparrow$}} \\ \cline{5-6}
     & & & & $\delta < 1.25$ & $\delta<1.25^2$ \\
    \hline 
    %  \multirow{4}{*}{NewCRF +\textit{align}} & \multirow{4}{*}{\rotatebox{90}{RGB}} 
        &  \multirow{4}{*}{\rotatebox{90}{NIR}} 
                          & Day   & 2.938 & 0.941 & 0.994 \\ 
        NeWCRF          & & Night & 2.937 & 0.922 & 0.994 \\ 
        +\textit{align} & & Rain  & 4.873 & 0.829 & 0.963 \\  \cline{3-6}
        & & \cellcolor{Gray1}Avg  & \cellcolor{Gray1}3.617 & \cellcolor{Gray1}0.896 & \cellcolor{Gray1}0.983 \\
    \midrule  
    %  \multirow{4}{*}{NewCRF +\textit{fuse}} & \multirow{4}{*}{\rotatebox{90}{RGB}} 
        & \multirow{4}{*}{\rotatebox{90}{NIR}} 
                         & Day   & 2.889 (\textcolor{red}{-0.049}) & 0.944 (\textcolor{red}{+0.003}) & 0.995 (\textcolor{red}{+0.001}) \\
        NeWCRF         & & Night & 2.840 (\textcolor{red}{{-0.097}}) & 0.931 (\textcolor{red}{{+0.009}}) & 0.994 (\textcolor{red}{{+0.000}}) \\
        +\textit{fuse}  & & Rain  & 3.975 (\textcolor{red}{\textbf{-0.898}}) & 0.879 (\textcolor{red}{\textbf{+0.050}}) & 0.981 (\textcolor{red}{\textbf{+0.018}}) \\ \cline{3-6}
        & & \cellcolor{Gray1}Avg  & \cellcolor{Gray1}3.255 (\textcolor{red}{-0.362})  & \cellcolor{Gray1}0.917 (\textcolor{red}{+0.021}) & \cellcolor{Gray1}0.990 (\textcolor{red}{+0.007}) \\
    \bottomrule
    \end{tabular} 
}
\end{center}
\label{tab:ablation3}
\end{table}

\begin{table}[t]
\centering
\caption{\textbf{The effect of multi-spectral feature fusion for various environments (Thermal).}  
To investigate the effect of multi-spectral feature fusion under each environmental condition, we compare evaluation results (\ie, Day, Night, and Rain).
GT depth maps projected to the thermal image plane are used for evaluation.
} \vspace{-0.1in}
\begin{center}
\resizebox{0.99\linewidth}{!}
{
    
    \footnotesize
    \begin{tabular}{c|c|c|c|cc} 
    \toprule
    \multirow{2}{*}{Method} & \multirow{2}{*}{Modal} & \multirow{2}{*}{TestSet} & \multirow{2}{*}{RMSE ($\downarrow)$} & \multicolumn{2}{c}{\textbf{Accuracy $\uparrow$}} \\ \cline{5-6}
     & & & & $\delta < 1.25$ & $\delta<1.25^2$ \\
    \hline 
    %  \multirow{4}{*}{NewCRF +\textit{align}} & \multirow{4}{*}{\rotatebox{90}{RGB}} 
        &  \multirow{4}{*}{\rotatebox{90}{THR}} 
                          & Day   & 2.671 & 0.954 & 0.995 \\ 
        NeWCRF          & & Night & 2.519 & 0.951 & 0.996 \\ 
        +\textit{align} & & Rain  & 3.349 & 0.916 & 0.990 \\  \cline{3-6}
        & & \cellcolor{Gray1}Avg  & \cellcolor{Gray1}2.860 & \cellcolor{Gray1}0.940 & \cellcolor{Gray1}0.994 \\
    \midrule  
    %  \multirow{4}{*}{NewCRF +\textit{fuse}} & \multirow{4}{*}{\rotatebox{90}{RGB}} 
        & \multirow{4}{*}{\rotatebox{90}{THR}} 
                         & Day   & 2.452 (\textcolor{red}{\textbf{-0.219}}) & 0.964 (\textcolor{red}{\textbf{+0.010}}) & 0.997 (\textcolor{red}{+0.002}) \\
        NeWCRF         & & Night & 2.424 (\textcolor{red}{{-0.095}}) & 0.960 (\textcolor{red}{{+0.009}}) & 0.998 (\textcolor{red}{{+0.002}}) \\
        +\textit{fuse}  & & Rain  & 2.964 (\textcolor{red}{\textbf{-0.385}}) & 0.939 (\textcolor{red}{\textbf{+0.023}}) & 0.994 (\textcolor{red}{\textbf{+0.004}}) \\ \cline{3-6}
        & & \cellcolor{Gray1}Avg  & \cellcolor{Gray1}2.623 (\textcolor{red}{-0.237})  & \cellcolor{Gray1}0.954 (\textcolor{red}{+0.014}) & \cellcolor{Gray1}0.996 (\textcolor{red}{+0.002}) \\
    \bottomrule
    \end{tabular} 
}
\end{center}
\label{tab:ablation4}
\end{table}
